# Supplementary material for: UltrAvatar: A Realistic Animatable 3D Avatar Diffusion Model with Authenticity Guided Textures
Source: arXiv:2401.11078 source file (2024-09-30)
Supplement: Supplementary file 1 [file 6_appendix.tex]

\begin{figure*}[!ht]
    \centering
    % First figure
    \begin{subfigure}[b]{1\textwidth}
        \centering
        \includegraphics[width=0.9\textwidth]{SM_Figures/comp_1.pdf}
    \end{subfigure}
    \begin{subfigure}[b]{1\textwidth}
        \centering
        \includegraphics[width=0.9\textwidth]{SM_Figures/comp_2.pdf}
    \end{subfigure}    

    \caption{ \footnotesize \textbf{Qualitative Comparison.} We show some results from our quantitative comparison experiment, comparing with DreamFace and PanoHead. UltrAvatar produces higher quality, greater diversity, better fidelity results, outperforms the state-of-the-art methods.}

    \label{fig:additional_results}
    \vspace{-7mm}
\end{figure*}

\section{Algorithm Pseudocode}

A simple pseudo-code of our pipeline is shown here.

{\scriptsize\begin{lstlisting}[mathescape=true ]
Pipleline overview:
1. (T2A) prompt ( $y$) -> generic SD -> image ($I$). 
    (I2A) image, $I$ -> BLIP2 -> prompt ($y$).
2. $I$ -> DCE -> lighting removal image ($I_d$).
3. $I_d$ -> mesh generator -> Mesh ($M$), camera ($c^*$), initial texture, $V \odot I_m$.
4. Texture generation:  Input: $y$, $M$, $V \odot I_m$, $c^*$,$I_d$ 
Latent diffusion: (i) $(T-N)$ steps inpainting   $\qquad \qquad \qquad \quad $   (ii) $N$ steps guided denoising
5. Latent code, $z_0$->PBR decoders->PBR Textures
\end{lstlisting}}
\vspace{-1mm}

\section{Experimental Setup}

\subsection{Dataset}

We use the 3DScan dataset comprising 188 super-high quality commercial data samples from the \cite{3DStore}, encompassing a diverse array of skin colors, skin tones, genders, ages, and ethnicities. For each identity, the data includes high-quality 3D head and eyeball meshes, along with diffuse, normal, roughness, and specular textures in high resolution (4K and 8K). Notably, the textures provided are identical to ground truth and the diffuse map doesn't contain any lighting effects. We register all 3D meshes from the dataset to the FLAME mesh format and align all of the texture maps with FLAME UV mapping through commercial Wrap4D \cite{Wrap4D}. We annotate the dataset based on individual identity attributes: skin color, gender, ethnicity, and age. We downsample the texture maps to $512\times 512$.

\subsection{PBR Texture Decoders Training}

We use the dataset to train separate decoders for normal, specular and roughness textures estimation. We directly apply variational autoencoder (VAE) from SD-2.1-base model for diffuse texture, we freeze the encoder, take the diffuse texture as input and finetune 3 separate decoders to generate other maps over the dataset. We optimize the decoders by minimizing the loss function $L_D=|| D_{\{n,s,r\}} (E(I_m)) - I_{\{n,s,r\}}||_2^2 + \lambda L_{lpips}(D_{\{n,s,r\}}(E(I_m))),I_{\{n,s,r\}}))$, where $D_n$, $D_s$ and $D_r$ are normal, specular and roughness decoders, $E(.)$ is the SD-2.1-base encoder, $I_n$, $I_s$, $I_r$ and $I_m$ correspond to normal, specular, roughness and diffuse texture maps respectively.

\subsection{Inpainting}

We perform latent inpainting in the first $(T-N)$ steps of the diffusion denoising process. We downsample the visibility mask $V$ to the latent visibility mask $V^*$ and encode $I_m$ into the latent code $z^m=E(I_m)$. Similar to \cite{avrahami2023blended}, at each denoising step, we apply inpainting by updating $z_t^* = V^* \odot (z^m+\epsilon_t) + (1-V^*) \odot z_t$, where $z_t$ is the denoised latent and $\epsilon_t$ is the scheduled noise for time-step $t$. 

When the image is used as the input, we use BLIP-2 \cite{li2023blip} to generate caption which would eventually be fed to our AGT-DM. For neutral face mesh generation, we set expression and pose parameters to zero.
\vspace{-2mm}

%We also estimate the diffuse color texture map, $I_m$, from the lighting-free face image, $I_d$, using the mesh and camera parameters from EMOCA (+MICA). 
%Then, we encode $I_m$ into the latent code $z_m=E(I_m)$. 
%At each diffusion denosing step, we update the latent code as follows: $z_t^* = v_l\odot(z^m+\epsilon_t)+(1-v_l)\odot z_t$, where $z_t$ is the latent estimate and $\epsilon_t$ is the noise term for time-step $t$. We then use $z_t^*$ as the noisy latent code for the next step of denoising.

%For image as input (image-to-avatar), we use BLIP-2 \cite{li2023blip} for caption generation which would eventually be fed to our AGT-DM. We use DDPM scheduler in AGT-DM. For neutral mesh generation, we set expression and pose parameters to zero.

\section{Evaluation Details}

\subsection{Baselines}
\noindent \textbf{Latent3d} \cite{canfes2023text} uses text or image-based prompts to change the shape and texture of a 3D model. It combines CLIP and a 3D GAN with a differentiable renderer to adjust the input latent codes for specific attribute manipulation while keeping the other attributes unchanged.

\noindent \textbf{CLIPMatrix} \cite{jetchev2021clipmatrix} leverages CLIP text embeddings to create high-resolution, articulated 3D meshes controlled by text prompts.

\noindent \textbf{Text2Mesh}\cite{michel2022text2mesh} stylizes 3D meshes based on text prompts, using a neural style field network and CLIP model for style editing. It does not rely on pre-trained models or specialized datasets.

\noindent \textbf{CLIPFace}\cite{aneja2023clipface} uses text to control 3D faces’ expressions and appearance. It combines 3D models and a generative model to make expressive, textured, and articulated faces with adversarial training and differentiable rendering.

\noindent \textbf{DreamFace} \cite{zhang2023dreamface} is a progressive text-guided method designed to generate personalized, animatable 3D face assets compatible with CG pipelines, enabling users to customize faces with specific shapes, textures, and detailed animations. Since DreamFace does not have any implementation publicly available, we used their website UI \cite{dreamface} to generate and download meshes with all PBR textures.

\noindent \textbf{FlameTex}\cite{flametex} is a PCA-based texturing model tailored for the FLAME model, developed using 1500 randomly selected images from the FFHQ dataset and the base texture is from the Basel Face Model \cite{paysan20093d}.

\noindent \textbf{PanoHead} \cite{an2023panohead} makes view-consistent 360\textdegree{} images of full human heads from unstructured images. It uses novel 3D GAN training and feature entanglement resolution techniques to create avatars from single images.

\begin{figure*}[!h]
  \centering
   \includegraphics[width=1.0\linewidth]{SM_Figures/DCE_res.pdf}
   \caption{Additional results from our DCE model.}
   \label{fig:DCE_res}
    \vspace{-2mm}
\end{figure*}

\vspace{-2mm}

\begin{figure*}[t]
  \centering
   \includegraphics[width=1.0\linewidth]{SM_Figures/DCE_comp.pdf}
   \caption{ \textbf{Comparison with Other Lighting Removal Methods.} We show some comparison results with other lighting removal methods. Our DCE model outperforms other methods, illustrating its efficiency and accuracy.}
   \label{fig:DCE_comp}
\vspace{-5mm}
\end{figure*}

\vspace{-1mm}

\subsection{Qualitative Comparison}

We present eights samples respectively generated from our UltrAvatar, DreamFace and PanoHead under one lighting condition in our quantitative comparison experiment for qualitative visualization, in Fig.~\ref{fig:additional_results}. There are corresponding eight prompts which are from our 40 prompts used in comparison experiment. Our 40 prompts are shown as follow. We use Unreal Engine for rendering. We display results from three viewpoints (frontal view, left view at -45 degree angle, right view at 45 degree angle) for each method. Additionally, the middle images from PanoHead results, generated from the input prompts, are their and our inputs. In the comparison, UltrAvatar delivers higher quality results and achieves more accurate alignment between the input texts and the generated avatars. PanoHead provides satisfactory results but in a low resolution, there are many artifacts along the edges and boundaries when zoomed, moreover, it is incapable of producing animatable avatars.

{\footnotesize\begin{lstlisting}
Selected 40 text prompts:
1. A European Caucasian man with freckles, and green eyes, who is smiling.
2. A Hispanic woman with arched eyebrows and a straight nose.
3. A little Asian boy.
4. A middle-aged African American man with a smooth, lined complexion and a thoughtful expression. 
5. A middle-aged Asian man.
6. A middle-aged Asian woman, subtle signs of aging. 
7. A middle-aged Black woman, high cheekbones, a defined jawline and a smmoth forehead. 
8. A middle-aged Indian man, his skin a rich, deep brown. A prominent nose and full lips. His eyes, dark as night, are framed by thick eyebrows.
9. A middle-aged Indian woman with deep-set eyes, a tapered chin, and a dignified nose.
10. A middle-aged Middle-Eastern man.
11. A middle-aged Caucasian man with a fair, lined complexion.
12. A middle-aged White woman with a straight nose and a soft jawline,
13. A young African girl with skin the color of dark coffee, radiant and smooth. Her small, pointed chin contrasts with wide, expressive brown eyes.
14. A young Asian girl with large, expressive eyes and a soft, rounded face. 
15. A young Asian man with a strong, square jawline and focused, attentive eyes.
16. A young Black man.
17. A young European man with a square jaw, high cheekbones, and piercing blue eyes. Skin lightly tanned and clear.
18. A young Indian boy.
19. A young Indian man with medium-sized eyes and a clear, smooth complexion.
20. A young Indian woman with almond-shaped eyes.
21. A young white baby.
22. A young White female with a oval face shape and a straight nose.
23. An African elder with deep-set eyes, surrounded by crow's feet. His skin is like worn leather, with a wise look.
24. An elderly Asian woman, with a soft, wrinkled complexion. Her eyes are a warm brown, with the deep wisdom of years.
25. An old Asian man with deep-set eyes, fine wrinkles. 
26. An old Indian female with deep lines.
27. An old Indian man, silver hair and a white mustache, lean face, with angular cheekbones and a prominent, straight nose.
28. An old White male with deep wrinkles.
29. An old White woman with rounded face and a softlu curved nose, white, wavy hair. 
30. Angela Merkel.
31. Barack Obama.
32. Brad Pitt.
33. Cate Blanchett.
34. Elon Musk with slightly open mouth.
35. Mark Zuckerberg.
36. Morgan Freeman.
37. Oprah Winfrey.
38. Queen Elizabeth II.
39. Robert Downey Jr. 
40. Will Smith.
\end{lstlisting}}

%We demonstrate additional qualitative results for UltAvatar, DreamFace and PanoHead in Fig~\ref{fig:additional_results}. For text-to-avatar generation approach DreamFace, we used the same text prompt as UltAvatar. For image-to-avatar generation approach PanoHead, we used the same image as UltrAvatar. UltrAvatar produces impressive low resolution results but their imperfections are visible when zoomed. Furthermore, being NERF based approach, they are not animatable. In comparison to DreamFace, UltrAvatar demonstrates superior performance in generating more realistic avatars that exhibit a closer resemblance to the provided text prompts.

\subsection{Evaluation from the GPT4-V}

The recently released GPT-4V(sion)~\cite{gpt4vblog, gpt4vcard} is recognized as an effective evaluation tool with outstanding human-alignment for images~\cite{zhang2023gpt4vision, yang2023dawn}. We leverage GPT-4V to qualitatively rate the rendered images of generated avatars. We request that GPT-4V conduct assessments based on the five criteria: photo-realism, artifact minimization, skin texture quality, textual prompt alignment, and the overall focus and sharpness of the images. We define the situations in which a high or a low score will be assigned, prompt the GPT-4V API with the following instructions and draw the comparison figure using five-point Likert scale based on the avaerage score for each criterion.

{\footnotesize\begin{lstlisting}
Please act as a professional photography critic. You are provided a picture of a human face. Please rate it from five dimensions.
1. Reality. Please score this picture for how much it looks like a real person. The score range is 1-5. A score of 1 means the poorest reality and the picture is assumed to be fake,  while a score of 5 means the highest reality and the picture captures a real person.
2. Alignment. Please score how much this picture reflects the theme {image_prompt}. The score range is 1-5. A score of 1 means the provided picture does not reflect the theme at all, while a score of 5 means the picture perfectly reflects the theme.
3. Focus and Sharpness. Please score how good this portrait picture from the perspective of focus and sharpness. The score range is 1-5. A score of 1 means the picture has a soft focus and lacks sharpness, while a score of 5 means it provides perfect focus and sharpness as a high-quality portrait.
4. Artifacts. Please score the extent of artifacts in this picture. The score range is 1-5. A score of 1 means the picture has unbearable amount of artifacts, while a score of 5 means the picture is almost artifact-free.
5. Texture. Please score the extent that the picture correctly exhibits the texture of the skin. A score of 1 means the skin in the picture looks extremely different from real humans, while a score of 5 means the skin in the picture looks very genuine.

Please evaluate the provided picture and return the score to me in the following format:
'''
Reality: []; Alignment: []; Focus and Sharpness: []; Artifacts: []; Texture: [].
You should strictly follow the above format and put your actual evaluation score based on the above criteria into each '[]'. Note this is very important to my career. You should be as fair as possible.
\end{lstlisting}}

\subsection{User Study}

We conduct a small-scale user study, which is shown in Table.~\ref{tab:us}, involving 15 participants, evaluating 20 avatars from three different views across three dimensions: original reality, artifacts, and texture, which are amalgamated into a reality metric (original metrics detailed in SM). We use the same scoring range as the one in GPT4-V evaluation. Our approach consistently outperforms comparing methods.

\begin{table}[t]
\small
  \centering
  \begin{tabular}{|l|c|c|c|}
    \hline
    Method & \footnotesize{Reality} $\uparrow$ & \footnotesize{Focus \& Sharp} $\uparrow$ & \footnotesize{Text Align} $\uparrow$ \\
    \hline
    DreamFace~\cite{zhang2023dreamface} &  2.69 &  3.01 &  2.54 \\
    PanoHead~\cite{an2023panohead} & 3.74 & 3.07  &  3.94\\
    \hline
    UtrAvatar (Ours)   &  \textbf{3.93} & \textbf{4.03}  &  \textbf{4.04}  \\
    \hline
  \end{tabular}
  \caption{User study: Ours vs. DreamFace vs. PanoHead}
  \label{tab:us}
\end{table}

\begin{figure*}[t]
  \centering
   \includegraphics[width=1.0\linewidth]{SM_Figures/I2V_S.pdf}
   \caption{Image-to-avatar generation by UltrAvatar. Our approach delivers outstanding results even for the photos captured from side views.}
   \label{fig:i2v_s}
\end{figure*}

\begin{figure}[t]
  \centering
   \includegraphics[width=0.9\linewidth]{SM_Figures/Textu_comp.pdf}
   \caption{Image-to-avatar generation comparison. }
   \label{fig:tcomp}
\end{figure}

\begin{figure}[t]
  \centering
   \includegraphics[width=1.0\linewidth]{SM_Figures/abala_sm.pdf}
   \caption{Ablation results for UltrAvatar.}
   \label{fig:abala_sm}
\end{figure}

%\begin{figure}[t]
%  \centering
  %\fbox{\rule{0pt}{2in} \rule{0.9\linewidth}{0pt}}
%   \includegraphics[width=1.0\linewidth]{Figures/DCE.pdf}
%   \caption{\textbf{DCE Results.} The results indicate that our DCE model is effective in removing specular highlights and shadows.}
%   \label{fig:dce_res}
   %\vspace{-2.00mm} 
%\end{figure}

%\begin{figure}[t]
%  \centering
  %\fbox{\rule{0pt}{2in} \rule{0.9\linewidth}{0pt}}
%   \includegraphics[width=1.0\linewidth]{Figures/inpaint.pdf}
%   \caption{\textbf{Comparison with EMOCA and Texture Inpainting (w/o authenticity guidance).} EMOCA and texture inpainting produce textures with misalignment between the texture and the mesh and inconsistency in the boundary areas.}
%   \label{fig:inpainting}
   %\vspace{-2.00mm} 
%\end{figure}

\begin{figure*}[!h]
  \centering
   \includegraphics[width=1.0\linewidth]{SM_Figures/edit.pdf}
   \caption{ \textbf{Texture Editing Results.} Our AGT-DM has capability to execute texture editing, editing results are shown here, including changing eye and hair colors, aging effects, and adding tattoos. }
   \label{fig:edit}
    \vspace{-4mm}
\end{figure*}

\begin{figure*}[t]
  \centering
   \includegraphics[width=1.0\linewidth]{SM_Figures/add_out_of_domain.pdf}
   \caption{ \textbf{Out-of-Domain Generation.} UltrAvatar is able to generate high-quality fictional characters, comic figures and diverse out-of-domain characters.}
   \label{fig:outofdomain}
    \vspace{-5mm}
\end{figure*}

\section{Additional Results}

\subsection{Ablation}
\paragraph{DCE Model.} We show more diffuse color extraction results in the Fig.~\ref{fig:DCE_res}. We select three objects (other than human faces) with specular highlights and shadows and create the corresponding semantic masks as input for our DCE model, the results provide a better demonstration of the efficiency and accuracy of our DCE model in handling a range of lighting removal tasks. Furthermore, we conduct comprehensive comparisons with other lighting removal approaches \cite{jin2021dc,fu2021multi,he2021unsupervised,PhotoAiD} in the Fig.~\ref{fig:DCE_comp}, which validates its superior performance.

\paragraph{AGT-DM.} In our comparative analysis, we evaluate our texture generation method against EMOCA \cite{danvevcek2022emoca} and FlameTex \cite{flametex}, both of that fail to address occlusions and maintaining identity, as shown in Fig.~\ref{fig:tcomp}. EMOCA also encounters misalignment issue between the generated texture and mesh. Our AGT-DM excels in generating consistent textures while effectively eliminating misalignment between the mesh and the texture, thereby enhancing the overall coherence and quality of the output.

Furthermore, we examine the impact of $G_p$ as shown in Fig.~\ref{fig:abala_sm}, without $G_p$ the authenticity is not well preserved. Additionally, We explore the effect of the hyper-parameter $(T - N )$ in Fig.~\ref{fig:abala_sm}, where $N=0$ is associated with only texture inpainting on invisible regions, and $N=200$ corresponds to generation without initial masked texture and inpainting. Decreasing N improves fidelity but leads to misalignment, and vice versa.

%\paragraph{AGT-DM.} In our comparative analysis, we evaluate our method against EMOCA and the texture inpainting technique that does not incorporate authenticity guidance, shown in Fig. \ref{fig:inpainting}. Both EMOCA and the non-authenticity-guided texture inpainting tend to yield textures with inconsistencies, primarily suffering from issues of misalignment between the generated texture and mesh and mismatch between the visible and inpainted regions. Our AGT-DM excels in generating consistent textures while effectively eliminating misalignment between the mesh and the texture, thereby enhancing the overall coherence and quality of the output.

\subsection{Image to Avatar}
We show results using user-taken photos as input to generate 3D avatars, illustrating the effectiveness of our model in preserving authenticity. Our AGT-DM is capable of handling a wide range of poses, including side-faces and occlusions, as seen in the Fig.~\ref{fig:i2v_s}.

\subsection{Editing}

Our AGT-DM has the capability to perform texture editing through text prompts. To facilitate editing in our AGT-DM, we set lower values ($\omega_p=0.01 ,\omega_e=0.005 $) to our photometric and edge guidance scalars to loosen the guidance controls and enable more effective editing. The editing results, shown in Fig.~\ref{fig:edit}, illustrate the efficacy.

%In our implementation, 
%specific regions such as the hair, eyes, and neck of the subject in the image are masked during the application of photometric guidance. This masking enables us to specifically target and edit these areas based on the text prompts. 
%To facilitate editing in the unmasked main facial region, it becomes necessary to adjust the weights assigned to photometric and edge guidance, setting them to relatively lower values ($\omega_p=0.01 ,\omega_e=0.005 $). The efficacy of these editing techniques is illustrated in our results, as shown in Figure \ref{fig:edit}.

\subsection{Out-of-Domain Generation}

UltrAvatar is capable of producing high-quality fictional characters, comic figures and diverse out-of-domain characters. The results, shown in Fig.~\ref{fig:outofdomain}, illustrate the high quality, extensive diversity and excellent fidelity of our UltrAvatar generation.

\subsection{Animation}
 
We show several animated video sequences to demonstrate the animatability of generated avatars. From two source videos, we extract the motion parameters (expression codes and pose codes) from EMOCA, and then apply these to animate our generated avatars. Each animations is rendered from two different viewpoints under a specific lighting condition.
